# Supplementary material for: Inelastic Neutron Scattering Analysis with Time-Dependent Gaussian-Field Models
Source: arXiv:2106.13688 source file (2021-06-25)
Supplement: Supplementary file 1 [file R1_SI.pdf]

**Supplemental Material:**

# Inelastic Neutron Scattering Analysis with Time-Dependent Gaussian-Field Models

Cedric J. Gommes,[1,a] Reiner Zorn,[1] Sebastian Jaksch,[2] Henrich Frielinghaus,[2] and Olaf Holderer[2]

[1] *Forschungszentrum Jülich GmbH, Jülich Center for Neutron Science, 52425 Jülich, Germany*

[2] *Forschungszentrum Jülich GmbH, Jülich Center for Neutron Science at the Heinz Maier Leibnitz Zentrum, Lichtenbergstrasse 1, 85747 Garching, Germany*

(Dated: 22 June 2021)

[a] Current affiliation: Department of Chemical Engineering, University of Liège B6A, allée du Six Août 3, B-4000, Liège, Belgium; Electronic mail: cedric.gommes@uliege.be

## CONTENTS

**I. Correlation function $C_\rho(r,\tau)$ of three-phase systems** 3

**II. Figures of fields GRF-1 to GRF-7 of Table I** 6

**III. Static field with piecewise-linear spectral density (GRF-8)** 10
A. Base functions in reciprocal and real spaces 11
B. Normalization of $f_n$ and $\langle q^2 \rangle$ 13
C. Fitting procedure 14

**IV. Dynamic model 2: $g_W(r,\tau)$ for linear and quadratic dispersion relations** 17
A. Linear dispersion relation 17
B. Quadratic dispersion relation 17

**V. Dynamic model 3: $g_W(r,\tau)$ for static field GRF-4 (deformation mode)** 19
A. Ballistic wave propagation 20
B. Diffusive wave propagation 20

**VI. Asymptotic expansion of the intermediate scattering function** 22

**VII. Influence of numerical parameters on the SANS and NSE analysis of the emulsion** 24
A. Shape of the dispersion relation 24
B. Asymptotic exponent $\nu$ of the piecewise-linear spectral density 24
C. Number of $q$ values 26

## I. CORRELATION FUNCTION $C_\rho(r,\tau)$ OF THREE-PHASE SYSTEMS

We consider a three-phase system, with phases A, B and C defined by their indicator functions $\mathcal{I}_A(\mathbf{x},t)$, $\mathcal{I}_B(\mathbf{x},t)$ and $\mathcal{I}_C(\mathbf{x},t)$. The indicator functions takes the value 1 if point $\mathbf{x}$ is in the corresponding phase at time $t$ and 0 otherwise. The three phases fill-up space, which reads

$$\mathcal{I}_A(\mathbf{x},t) + \mathcal{I}_B(\mathbf{x},t) + \mathcal{I}_C(\mathbf{x},t) = 1 \tag{SM-1}$$

for any $\mathbf{x}$ and $t$.

The volume fraction of any phase is

$$\phi_X = \langle \mathcal{I}_X(\mathbf{x},t) \rangle \tag{SM-2}$$

where the brackets stand for averages over $\mathbf{x}$ (or ensemble averages), and the covariances are defined as

$$C_{XY}(\mathbf{r},\tau) = \langle \mathcal{I}_X(\mathbf{x},t)\mathcal{I}_Y(\mathbf{x}+\mathbf{r},t+\tau) \rangle \tag{SM-3}$$

where $X$ and $Y$ can be any of A, B, or C. All models considered in the main text are stationary in both space and time, so that the volume fractions are independent of space and time, and the covariances depend only on the space and times differences $\mathbf{r}$ and $\tau$.

In absence of long-range correlation, the covariances satisfy

$$C_{XX}(r \to \infty, \tau) = \phi_X^2 \tag{SM-4}$$

$$C_{XY}(r \to \infty, \tau) = \phi_X \phi_Y \tag{SM-5}$$

which express the statistical independence of $\mathcal{I}_X(\mathbf{x},t_1)$ and $\mathcal{I}_Y(\mathbf{x}+\mathbf{r},t_2)$ for large $|\mathbf{r}|$, and any times $t_1$ and $t_2$.

A total of six self- and cross-covariances can be defined for a three-phase system: $C_{AA}$, $C_{BB}$, $C_{CC}$, $C_{AB} = C_{BA}$, $C_{AC} = C_{CA}$ and $C_{BC} = C_{CB}$. These covariances, however, are not independent because they are linearly related to each other

$$C_{AA}(\mathbf{r},\tau) + C_{AB}(\mathbf{r},\tau) + C_{AC}(\mathbf{r},\tau) = \phi_A \tag{SM-6}$$

$$C_{BA}(\mathbf{r},\tau) + C_{BB}(\mathbf{r},\tau) + C_{BC}(\mathbf{r},\tau) = \phi_B \tag{SM-7}$$

$$C_{CA}(\mathbf{r},\tau) + C_{CB}(\mathbf{r},\tau) + C_{CC}(\mathbf{r},\tau) = \phi_C \tag{SM-8}$$

which result from Eqs. (SM-1) and (SM-3). As a consequence, all self-covariances can be expressed in terms of cross-covariances

$$C_{AA} = \phi_A - C_{AB} - C_{AC} \tag{SM-9}$$

with all possible permutations of A, B and C. And any cross-covariance can be expressed in terms of self-covariances

$$C_{AB} = \frac{1}{2}(\phi_A + \phi_B - \phi_C) - \frac{1}{2}(C_{AA} + C_{BB} - C_{CC}) \tag{SM-10}$$

with all possible permutations of A, B and C.

The scattering length densities of the three phases are $\rho_A$, $\rho_B$ and $\rho_C$, so that the scattering length density function is piecewise-constant

$$\rho(\mathbf{x}, t) = \rho_A \mathcal{I}_A(\mathbf{x}, t) + \rho_B \mathcal{I}_B(\mathbf{x}, t) + \rho_C \mathcal{I}_C(\mathbf{x}, t) \tag{SM-11}$$

and the average scattering length is

$$\langle \rho \rangle = \rho_A \phi_A + \rho_B \phi_B + \rho_C \phi_C \tag{SM-12}$$

The correlation function of the scattering-length density is

$$C_\rho(\mathbf{r}, \tau) = \langle \rho(\mathbf{x}, t) \rho(\mathbf{x} + \mathbf{r}, t + \tau) \rangle \tag{SM-13}$$

which can be written as

$$\begin{aligned} C_\rho = {} & \rho_A^2 C_{AA} + \rho_A^2 C_{AA} + \rho_A^2 C_{AA} \\ & + 2\rho_A \rho_B C_{AB} + 2\rho_A \rho_C C_{AC} + 2\rho_B \rho_C C_{BC} \end{aligned} \tag{SM-14}$$

Using Eq. (SM-10) this can be written in terms of self-covariances only as

$$\begin{aligned} C_\rho = {} & (\rho_A - \rho_C)(\rho_A - \rho_B) C_{AA} + (\rho_B - \rho_A)(\rho_B - \rho_C) C_{BB} \\ & + (\rho_C - \rho_A)(\rho_C - \rho_B) C_{CC} \\ & + \phi_A(\rho_A \rho_B + \rho_A \rho_C - \rho_B \rho_C) + \phi_B(\rho_A \rho_B + \rho_B \rho_C - \rho_A \rho_C) \\ & + \phi_C(\rho_A \rho_C + \rho_B \rho_C - \rho_A \rho_B) \end{aligned} \tag{SM-15}$$

Evaluating the left and right sides for $r \to \infty$, with the help of Eqs. (SM-4) and (SM-5), and then subtracting them from the original equation leads to

$$\begin{aligned} C_\rho - \langle \rho \rangle^2 &= (\rho_A - \rho_C)(\rho_C - \rho_B)(C_{AA} - \phi_A^2) \\ &+ (\rho_B - \rho_A)(\rho_B - \rho_C)(C_{BB} - \phi_B^2) \\ &+ (\rho_C - \rho_A)(\rho_C - \rho_B)(C_{CC} - \phi_C^2) \end{aligned} \tag{SM-16}$$

which is Eq. 3 of the main text.

Similarly $C_\rho$ can also be calculated from Eq. (SM-9). This leads to

$$\begin{aligned} C_\rho - \langle \rho \rangle^2 &= (\rho_A - \rho_B)^2(\phi_A \phi_B - C_{AB}) \\ &+ (\rho_A - \rho_C)^2(\phi_A \phi_C - C_{AC}) \\ &+ (\rho_B - \rho_C)^2(\phi_B \phi_C - C_{BC}) \end{aligned} \tag{SM-17}$$

which contains only cross-covariances.

## II. FIGURES OF FIELDS GRF-1 TO GRF-7 OF TABLE I

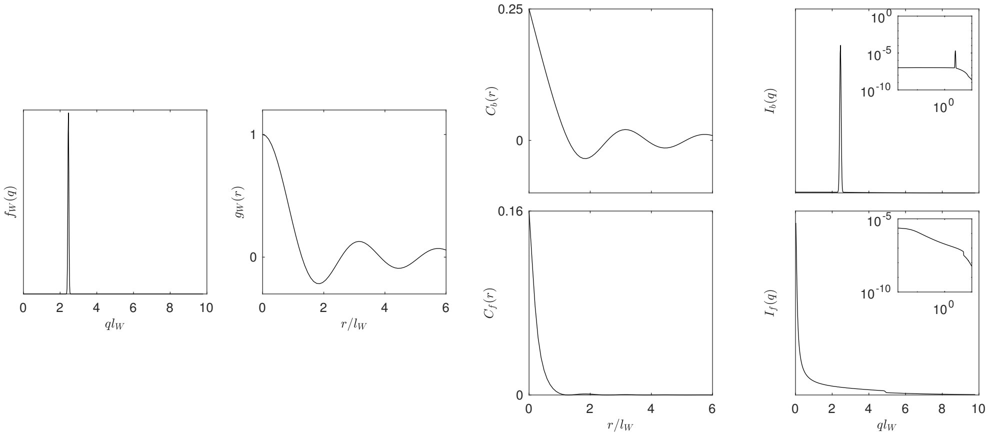


FIG. SM-1: Static Gaussian field GRF-1 from Table 1 of the main text. From left to right: spectral density $f_W(q)$, field correlation function $g_W(r)$, covariances $C_b(r)$ and $C_f(r)$ corresponding to bulk contrast ($\alpha = 0$, $\beta \to \infty$) and film contrasts ($\alpha = -0.25$ and $\beta = +0.25$), as well as scattering functions $I_b(q)$ and $I_f(q)$ obtained as the Fourier transform of the latter. The insets display the same data on double logarithmic scale.

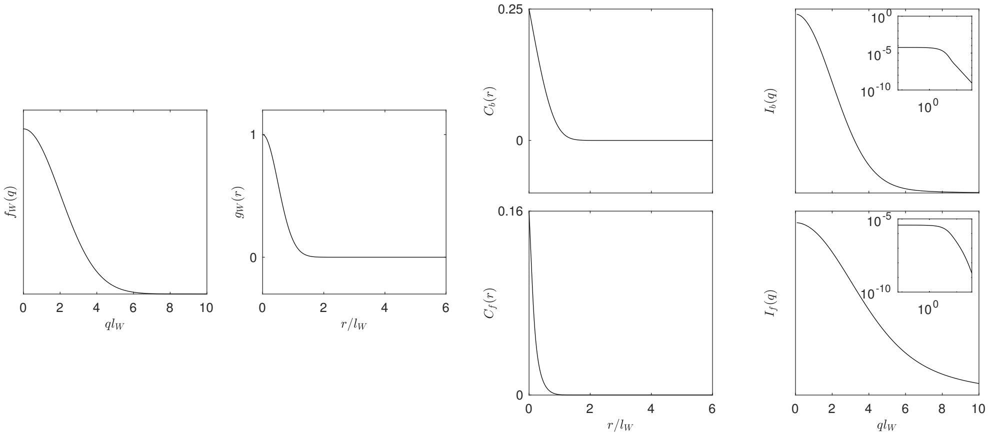


FIG. SM-2: Static Gaussian field GRF-2 from Table 1 of the main text. From left to right: spectral density $f_W(q)$, field correlation function $g_W(r)$, covariances $C_b(r)$ and $C_f(r)$ corresponding to bulk contrast ($\alpha = 0$, $\beta \to \infty$) and film contrasts ($\alpha = -0.25$ and $\beta = +0.25$), as well as scattering functions $I_b(q)$ and $I_f(q)$ obtained as the Fourier transform of the latter. The insets display the same data on double logarithmic scale.

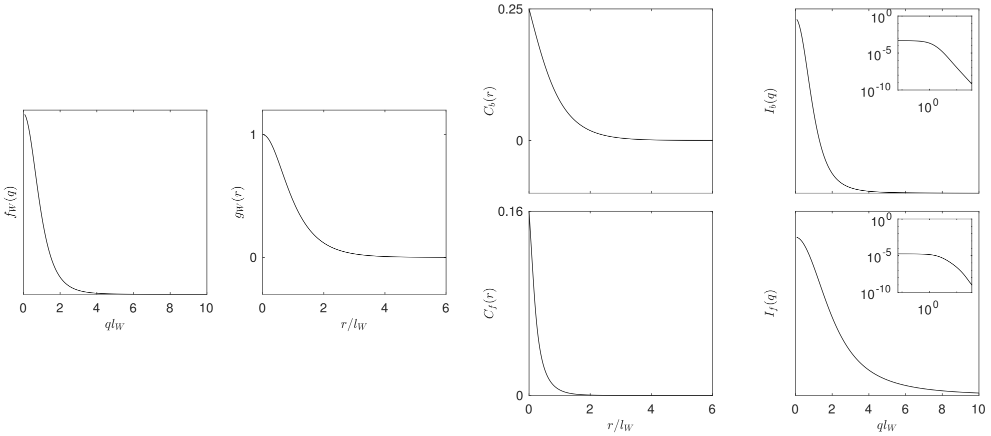


FIG. SM-3: Static Gaussian field GRF-3 from Table 1 of the main text. From left to right: spectral density $f_W(q)$, field correlation function $g_W(r)$, covariances $C_b(r)$ and $C_f(r)$ corresponding to bulk contrast ($\alpha = 0$, $\beta \to \infty$) and film contrasts ($\alpha = -0.25$ and $\beta = +0.25$), as well as scattering functions $I_b(q)$ and $I_f(q)$ obtained as the Fourier transform of the latter. The insets display the same data on double logarithmic scale.

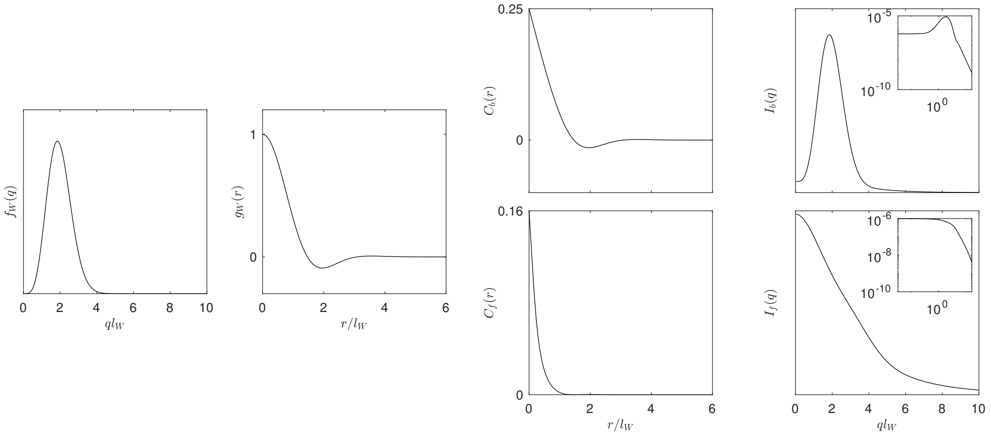


FIG. SM-4: Static Gaussian field GRF-4 from Table 1 of the main text. From left to right: spectral density $f_W(q)$, field correlation function $g_W(r)$, covariances $C_b(r)$ and $C_f(r)$ corresponding to bulk contrast ($\alpha = 0$, $\beta \to \infty$) and film contrasts ($\alpha = -0.25$ and $\beta = +0.25$), as well as scattering functions $I_b(q)$ and $I_f(q)$ obtained as the Fourier transform of the latter. The insets display the same data on double logarithmic scale.

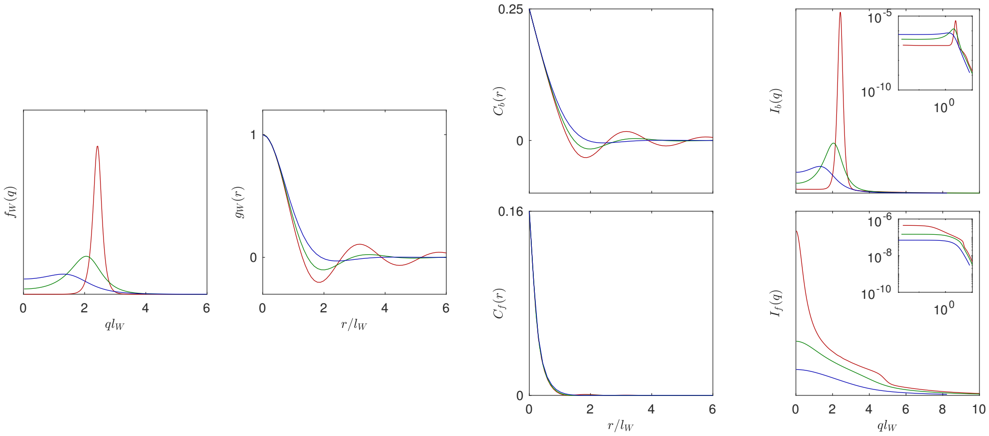


FIG. SM-5: Static Gaussian field GRF-5 from Table 1 of the main text, with $\mu = 0.5$ (red), $\mu = 2$ (green) and $\mu = 4$ (blue). From left to right: spectral density $f_W(q)$, field correlation function $g_W(r)$, covariances $C_b(r)$ and $C_f(r)$ corresponding to bulk contrast ($\alpha = 0$, $\beta \to \infty$) and film contrasts ($\alpha = -0.25$ and $\beta = +0.25$), as well as scattering functions $I_b(q)$ and $I_f(q)$ obtained as the Fourier transform of the latter. The insets display the same data on double logarithmic scale.

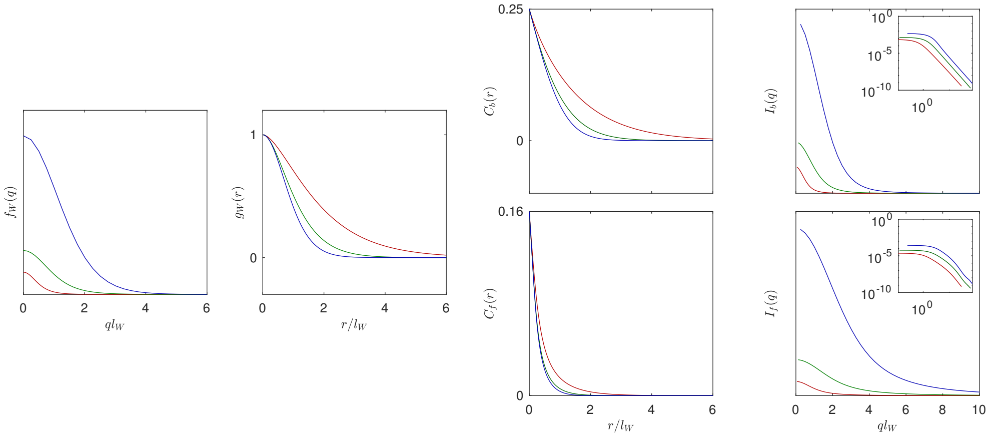


FIG. SM-6: Static Gaussian field GRF-6 from Table 1 of the main text, with $\mu = 1.2$ (red), $\mu = 2$ (green) and $\mu = 5$ (blue). From left to right: spectral density $f_W(q)$, field correlation function $g_W(r)$, covariances $C_b(r)$ and $C_f(r)$ corresponding to bulk contrast ($\alpha = 0$, $\beta \to \infty$) and film contrasts ($\alpha = -0.25$ and $\beta = +0.25$), as well as scattering functions $I_b(q)$ and $I_f(q)$ obtained as the Fourier transform of the latter. The insets display the same data on double logarithmic scale.

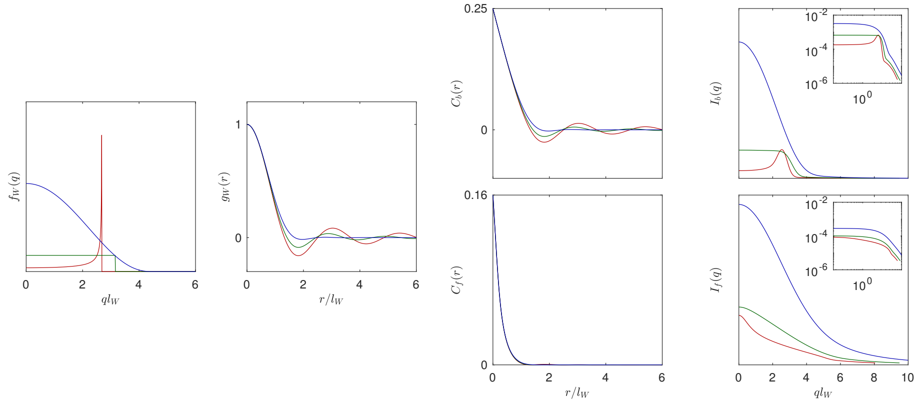

FIG. SM-7: Static Gaussian field GRF-7 from Table 1 of the main text, with $\mu = 0.8$ (red), $\mu = 1.5$ (green) and $\mu = 4$ (blue). From left to right: spectral density $f_W(q)$, field correlation function $g_W(r)$, covariances $C_b(r)$ and $C_f(r)$ corresponding to bulk contrast ($\alpha = 0$, $\beta \to \infty$) and film contrasts ($\alpha = -0.25$ and $\beta = +0.25$), as well as scattering functions $I_b(q)$ and $I_f(q)$ obtained as the Fourier transform of the latter. The insets display the same data on double logarithmic scale.

## III. STATIC FIELD WITH PIECEWISE-LINEAR SPECTRAL DENSITY (GRF-8)

The approach is sketched in Fig. SM-8. The spectral density is decomposed on a few piecewise linear base functions that interpolate between the values of $f(q)$ at a series of $N$ nodes with positions $q_n$ for $n = 1, \ldots, N$. We write formally

$$f_W(q) = \sum_{n=1}^{N} f_n \left(L_n(q) + R_n(q)\right) \tag{SM-18}$$

where $f_n$ is the value at the n$^{th}$ node and the base functions $L_n$ and $R_n$ are defined on the left and right sides of the node. For the right-handed side of the rightmost base function, a power-law is assumed with exponent $\nu$. Typically, the user chooses the positions of the nodes and the asymptotic exponent $\nu$, and the values $f_n$ are then considered as the fitting parameters of the model.

The field correlation function $g_W(r)$ is obtained as the Fourier transform of $f_W(q)$, namely

$$g_W(r) = \sum_{n=1}^{N} f_n \left(\tilde{L}_n(r) + \tilde{R}_n(r)\right) \tag{SM-19}$$

where

$$\tilde{R}/\tilde{L}_n(r) = \int_0^\infty R/L_n(q) \frac{\sin(qr)}{qr} 4\pi q^2 dq \tag{SM-20}$$

are the Fourier transforms of the right and left sides of the base functions. The expressions of $\tilde{L}$ and $\tilde{R}$ are given in Sec. III A.

The values of $f_n$ are subject to the constraint that the spectral density is normalized to one, namely

$$\int_0^\infty f_W(q) 4\pi q^2 \mathrm{d}q = 1 \tag{SM-21}$$

which is equivalent to ensuring $g_W(0) = 1$. This puts a linear constraint on $f_n$, given explicitly in Eq. (SM-34).

The field characteristic length $l_W$ is related to the second moment of $f_W(q)$ via

$$\frac{1}{l_W^2} = \frac{\langle q^2 \rangle}{6} \tag{SM-22}$$

with

$$\langle q^2 \rangle = \int_0^\infty f_W(q) q^2 \; 4\pi q^2 \mathrm{d}q \tag{SM-23}$$

The explicit expression for $\langle q^2 \rangle$ in terms of $f_n$ is derived in Eq. (SM-39).

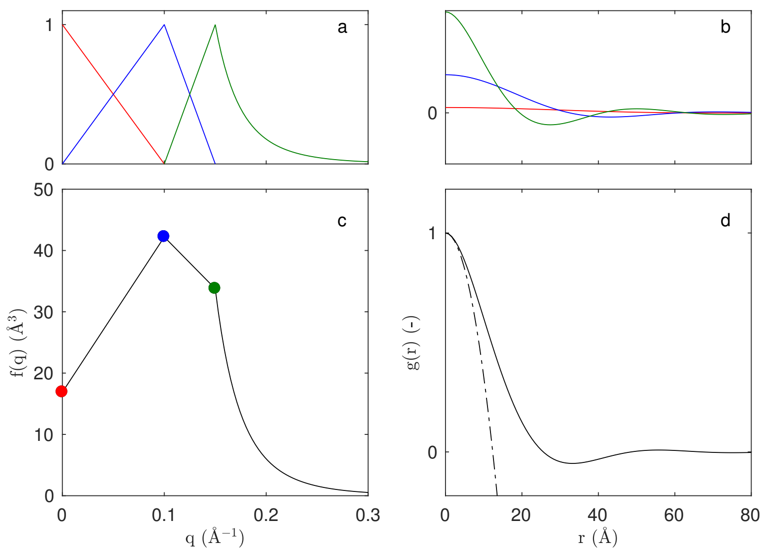


FIG. SM-8: Modelling of a GRF with piecewise-linear spectral density: base functions (a) and their corresponding contributions to the field correlation function (b), together with the full spectral density (c), and field correlation function (d). In all plots, the same colour code is used to highlight the same parameters. Case of $\nu = 6$; the quadratic behavior of $g_W(r)$ at the origin is highlighted with a dashed line.

## A. Base functions in reciprocal and real spaces

For all nodes except the first one ($1 < n \leq N$) the base function on the left of each node is linear

$$L_n(q) = (q - q_{n-1})/(q_n - q_{n-1}) \tag{SM-24}$$

For all nodes except the last one, the base function on the right of each node is linear

$$R_n(q) = (q_n - q)/(q_n - q_{n+1}) \tag{SM-25}$$

These functions ensure that $f_W(q)$ is continuous and piecewise-linear in the interval $[q_1, q_N]$. For the last node, its left-hand function $L_N(q)$ is identical to Eq. (SM-24), but we assume a power law on its right-hand side, namely

$$R_N = (q/q_N)^{-\nu} \tag{SM-26}$$

where the exponent $\nu$ is a parameter of the model. Note that integrability of $f_W(q)$ requires $\nu > 3$.

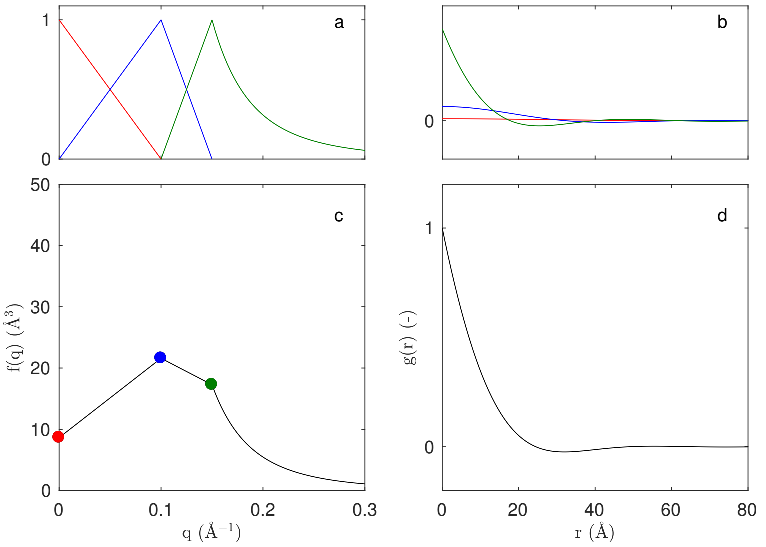


FIG. SM-9: Modelling of a GRF with piecewise-linear spectral density: base functions (a) and their corresponding contributions to the field correlation function (b), together with the full spectral density (c), and field correlation function (d). In all plots, the same colour code is used to highlight the same parameters. Case of $\nu = 4$, yielding a non-quadratic behavior of $g_W(r)$ at the origin.

For inner nodes, Eqs. (SM-24) and (SM-25), the Fourier transforms are

$$\tilde{L}_n(r) = \frac{4\pi}{r}\Delta\Big[\sin(q_{n-1}r)\left\{q_{n-1}C_1[\Delta r] + \Delta C_2[\Delta r]\right\} + \cos(q_{n-1}r)\left\{q_{n-1}S_1[\Delta r] + \Delta S_2[\Delta r]\right\}\Big] \tag{SM-27}$$

with $\Delta = q_n - q_{n-1}$, and

$$\tilde{R}_n(r) = \frac{4\pi}{r}\Delta\Big[\sin(q_n r)\left\{q_n C_0[\Delta r] + (\Delta - q_n)C_1[\Delta r] - \Delta C_2[\Delta r]\right\} + \cos(q_n r)\left\{q_n S_0[\Delta r] + (\Delta - q_n)S_1[\Delta r] - \Delta S_2[\Delta r]\right\}\Big] \tag{SM-28}$$

with $\Delta = q_{n+1} - q_n$, and

$$\begin{aligned} C_0[a] &= \int_0^1 \cos(ax)\ \mathrm{d}x = \frac{\sin(a)}{a} \\ C_1[a] &= \int_0^1 \cos(ax)x\ \mathrm{d}x = \frac{a\sin(a) + \cos(a) - 1}{a^2} \\ C_2[a] &= \int_0^1 \cos(ax)x^2\ \mathrm{d}x = \frac{2a\cos(a) + (a^2-2)\sin(a)}{a^3} \end{aligned} \tag{SM-29}$$

and

$$S_0[a] = \int_0^1 \sin(ax)\ \mathrm{d}x = \frac{1 - \cos(a)}{a}$$

$$S_1[a] = \int_0^1 \sin(ax)x \; \mathrm{d}x = \frac{\sin(a) - a\cos(a)}{a^2}$$
$$S_2[a] = \int_0^1 \cos(ax)x^2 \; \mathrm{d}x = \frac{2(a\sin(a) - 1) - (a^2 - 2)\cos(a)}{a^3} \quad \text{(SM-30)}$$

And for the right-hand base function of the last node, the Fourier transform is

$$\tilde{R}_N(r) = \frac{4\pi}{r^3}(q_N r)^\nu \mathrm{Re}\Big\{ i^{\nu-1}\Gamma\left(2-\nu, iq_N r\right) \Big\} \quad \text{(SM-31)}$$

where $\Gamma()$ is the (upper) incomplete gamma function. For the particular case $\nu = 6$

$$\tilde{R}_N(r) = \frac{\pi q_N^3}{6rq_N}\Big[(q_N r)^4\left(\frac{\pi}{2} - \mathrm{Si}(q_N r)\right)$$
$$-\big((q_N r)^2 - 6\big)\sin(q_N r) - (q_N r)\big((q_N r)^2 - 2\big)\cos(q_N r)\Big] \quad \text{(SM-32)}$$

where Si is the integral sine function. In all cases

$$\tilde{R}_N(r \to 0) = \frac{4\pi q_N^3}{\nu - 3} \quad \text{(SM-33)}$$

which shows again that $\nu$ has to be larger than 3.

## B. Normalization of $f_n$ and $\langle q^2 \rangle$

The normalization of $f_W(q)$ to one can be put as

$$\tilde{R}_1(0)f_1 + \sum_{n=2}^{N}\left(\tilde{L}_n(0) + \tilde{R}_n(0)\right)f_n = 1 \quad \text{(SM-34)}$$

where

$$\tilde{R}/\tilde{L}_n^{(0)} = \int_0^\infty \tilde{R}/\tilde{L}_n(q)4\pi q^2 dq \quad \text{(SM-35)}$$

are equal to the Fourier transforms of $R_n(q)$ and $L_n(q)$ evaluated at $r = 0$.

The explicit values are

$$\tilde{L}_n(0) = 4\pi\Delta\left[\frac{1}{2}(q_n - \Delta)^2 + \frac{2}{3}\Delta(q_n - \Delta) + \frac{1}{4}\Delta^2\right] \quad \text{(SM-36)}$$

with $\Delta = q_n - q_{n-1}$ and

$$\tilde{R}_n(0) = 4\pi\Delta\left[\frac{1}{2}q_n^2 + \frac{1}{3}\Delta q_n + \frac{1}{12}\Delta^2\right] \quad \text{(SM-37)}$$

with $\Delta = q_{n+1} - q_n$. For the last node

$$\tilde{R}_N(0) = \frac{4\pi q_N^3}{\nu - 3} \quad \text{(SM-38)}$$

The second moment of the spectral density $\langle q^2 \rangle$ is calculated as

$$\langle q^2 \rangle = \tilde{R}_n^{(2)} f_1 + \sum_{n=2}^{N} \left( \tilde{L}_n^{(2)} + \tilde{R}_n^{(2)} \right) f_n \qquad \text{(SM-39)}$$

where

$$\tilde{R}/\tilde{L}_n^{(2)} = \int_0^\infty q^2 \tilde{R}/\tilde{L}_n(q) 4\pi q^2 dq \qquad \text{(SM-40)}$$

are the second moments of the base functions.

For the left-hand base functions the values are

$$\begin{aligned} \tilde{L}_n^{(2)} = 4\pi\Delta \Big[ & \frac{1}{2}(q_n - \Delta)^4 + \frac{4}{3}\Delta(q_n - \Delta)^3 \\ & + \frac{3}{2}\Delta^2(q_n - \Delta)^2 + \frac{4}{5}\Delta^3(q_n - \Delta) + \frac{1}{6}\Delta^2 \Big] \end{aligned} \qquad \text{(SM-41)}$$

with $\Delta = q_n - q_{n-1}$. For the right-hand base functions

$$\begin{aligned} \tilde{R}_n^{(2)} = 4\pi\Delta \Big[ & \frac{1}{2}q_n^4 + \frac{2}{3}\Delta q_n^3 + \frac{1}{2}\Delta^2 q_n^2 \\ & + \frac{1}{5}\Delta^3 q_n + \frac{1}{30}\Delta^4 \Big] \end{aligned} \qquad \text{(SM-42)}$$

with $\Delta = q_{n+1} - q_n$. And for the last node

$$\tilde{R}_N^{(2)} = \frac{4\pi q_N^5}{\nu - 5} \qquad \text{(SM-43)}$$

Note that $\langle q^2 \rangle$ and $l_W$ are not defined for values smaller than $\nu = 5$.

## C. Fitting procedure

Typically, about $M \simeq 30 - 50$ nodes are chosen uniformly spaced from $q = 0$ to $q = 0.15$ Å$^{-1}$. For all cases considered in the main text, the asymptotic exponent $\nu = 6$ was chosen. From the position of the nodes and the value of $\nu$, the functions $\tilde{L}_n(r)$ and $\tilde{R}(r)$ are evaluated (see Eq. SM-19) and added to form $G_m(r)$ such that

$$g_W(r) = \sum_{m=1}^{M} G_m(r) f_m \qquad \text{(SM-44)}$$

The fitting parameters of the model are the values of spectral density $f_m$ at the nodes, which form a vector $\mathbf{f}$. In practice, the values of $G_m(r)$ are evaluated for about 500 distances from 0 to $5/\sigma_q$ (where $\sigma_q$ is the resolution of the instrument) and stored in a matrix $\underline{G}$ that is calculated once and for all, and handled as a global variable.

The clipping functions, which are used to convert the field correlation function $g_W(r)$ to the covariances $C_{oo}(r)$ or $C_{ss}(r)$ (see Fig. 3 of the main text), are also calculated once and for all, over about 100 values of $g_W$ from $-1/2$ to 1, for the values of $\alpha$ and $\beta$ that are relevant to bulk and film contrasts. The relevant values are stored in a matrix $\underline{C}$; whenever the covariances have to be evaluated from $g_W$, the values in the matrix are interpolated.

The evaluation of the scattered intensity proceeds as follows for any value of the parameters $\mathbf{f}$

1. The field correlation at all relevant values of $r$ is calculated as a matrix multiplication : $\mathbf{g} = \underline{G} \times \mathbf{f}$;

2. The values of $\underline{C}$ for all relevant values of $r$ are obtained from $\mathbf{g}$ via interpolation of $\underline{C}$, yielding the covariances $\mathbf{C}_b$ and $\mathbf{C}_f$ for bulk and film contrast;

3. The values of $\mathbf{C}_b$ and $\mathbf{C}_f$ are multiplied by the resolution function

$$\left(\frac{\sigma_q}{\sqrt{2\pi}}\right)^3 \exp\left[-\frac{(\sigma_q r)^2}{2}\right] \tag{SM-45}$$

   and Fourier-transformed (Eq. 4 of the main text) for each value of $q$. In practice this third step is also calculated as a matrix multiplication, with a Fourier matrix $\underline{F}$ that is also calculated once and for all.

The so-calculated values at $q(n_q)$ are referred to hereafter as $I_b(n_q;\mathbf{f})$ and $I_f(n_q;\mathbf{f})$.

Starting from the experimental scattered intensities $\hat{I}_b$ and $\hat{I}_f$ in bulk and film contrasts, the fitting is done by minimizing the following function

$$\begin{aligned}\chi^2(\mathbf{f}) = &\sum_{n_q=1}^{N_q} \frac{1}{\sigma_b^2(n_q)} \left(\hat{I}_b(n_q) - A_b I_b(n_q;\mathbf{f})\right)^2 \\ &+ \sum_{n_q=1}^{N_q} \frac{1}{\sigma_f^2(n_q)} \left(\hat{I}_f(n_q) - A_f I_f(n_q;\mathbf{f})\right)^2\end{aligned} \tag{SM-46}$$

where and $\sigma_b$ and $\sigma_f$ are the corresponding standard deviations. For any value of $\mathbf{f}$, the values of the factors $A_b$ and $A_f$ are obtained by setting

$$A_b = \left(\sum_{n_q} I_b(n_q)\hat{I}_b(n_q)/\sigma_b^2(n_q)\right) / \left(\sum_{n_q} I_b^2(n_q)/\sigma_b^2(n_q)\right) \tag{SM-47}$$

and the equivalent relation for $A_f$. These values result from setting $\partial\chi^2/\partial A_b = 0$ and $\partial\chi^2/\partial A_f = 0$. The minimization of $\chi^2$ on the remaining parameters $\mathbf{f}$ is performed in Matlab, using the function "fmincon" subject to the linear constraint $\sum_n G_n(0) f_n = 1$ (see Eq. SM-34).

Examples of fits for increasing number of nodes are illustrated in Fig. SM-10, using the SANS data of the main text. The values for $N = 50$ is used throughout the main text.

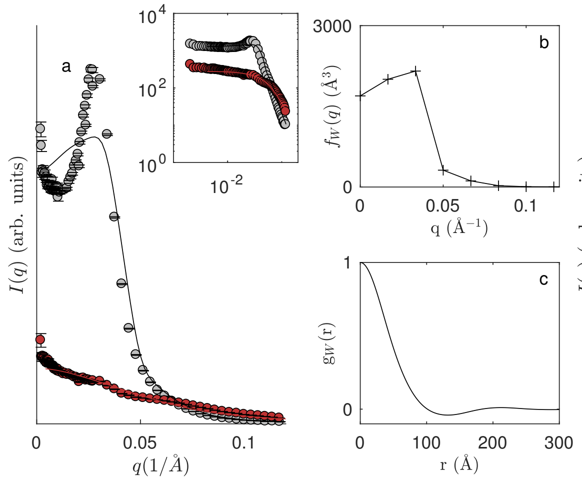


(a) $N = 10$

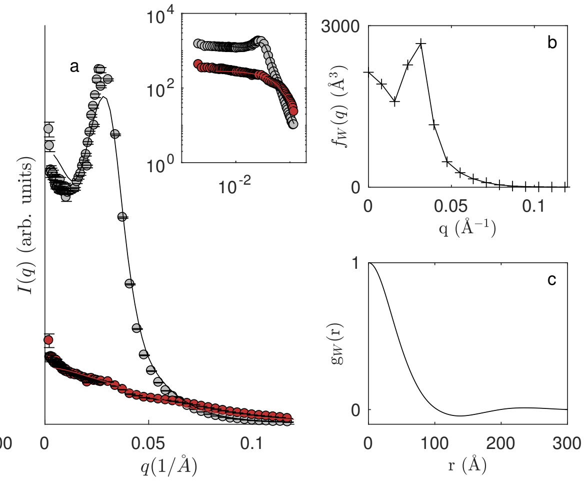


(b) $N = 20$

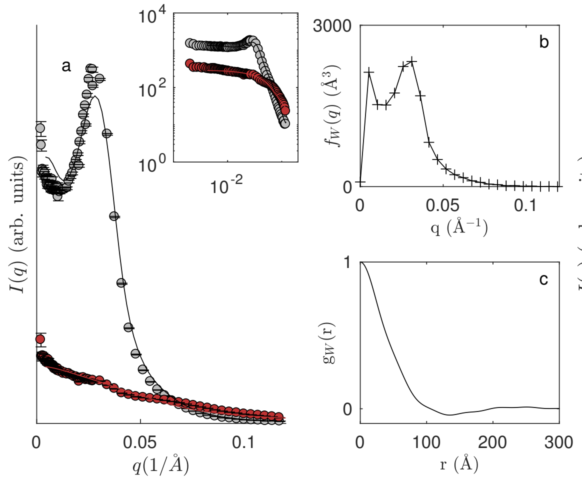


(c) $N = 30$

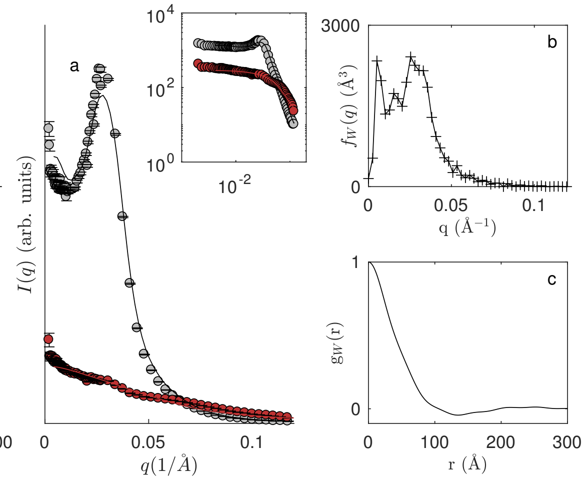


(d) $N = 60$

FIG. SM-10: Illustration of the number of nodes $N$ for the fitting of the piecewise-linear model to the SANS data of the main text. In each case: (a) Joint fit of the bulk-contrast (grey) and film-contrast (red) emulsion data; (b) corresponding spectral density with nodes shown as crosses, and (c) corresponding field correlation function.

## IV. DYNAMIC MODEL 2: $g_W(r,\tau)$ FOR LINEAR AND QUADRATIC DISPERSION RELATIONS

### A. Linear dispersion relation

In the case of a linear dispersion relation $\omega = cq$, the correlation function $g_W(r,\tau)$ is obtained easily from the static correlation function $g_W(r,0)$. The relation between $g_W(r,0)$ and $f_W(q)$ is indeed an inverse Fourier transform, namely

$$\frac{r}{4\pi} g(r,0) = \int_0^\infty f(q)\sin(qr)q\mathrm{d}q \tag{SM-48}$$

On the other hand, Eq. (35) of the main text can be written as

$$g(r,\tau) = \frac{2\pi}{r}\int_0^\infty f(q)\left[\sin(q(r+c\tau)) + \sin(q(r-c\tau))\right] q\mathrm{d}q \tag{SM-49}$$

is the particular case of $\omega = c\tau$. This leads to the general relation

$$\begin{aligned} g_W(r,\tau) = &\frac{1}{2}\left[g_W(r+c\tau,0) + g_W(r-c\tau,0)\right] \\ &+ \frac{c\tau}{2r}\left[g_W(r+c\tau,0) - g_W(r-c\tau,0)\right] \end{aligned} \tag{SM-50}$$

which is valid for any $f_W(q)$ or $g_W(r)$.

In the particular case of static field GRF-2 of Tab. I from the main text, with

$$g_W(r) = \exp\left[-\left(\frac{r}{l}\right)^2\right] \tag{SM-51}$$

the correlation function becomes

$$\begin{aligned} g_W(r,\tau) = \exp\left[-\frac{r^2+(c\tau)^2}{l^2}\right] \times \\ \left\{\cosh\left[\frac{2rc\tau}{l^2}\right] - 2\left(\frac{c\tau}{l}\right)^2 \sinh\left[\frac{2rc\tau}{l^2}\right] / \left[\frac{2rc\tau}{l^2}\right]\right\} \end{aligned} \tag{SM-52}$$

which proves Eq. (36) of the main text.

### B. Quadratic dispersion relation

In the case of a quadratic dispersion relation, $\omega = Dq^2$, no simple general relation comparable to Eq. (SM-50) can be obtained.

In the particular case of static field GRF-2 (see Eq. SM-51), however, Eq. (35) of the main text can be written as

$$g_W(r,\tau) = \frac{l^3}{(4\pi)^{3/2}} \times Re\left\{\int_0^\infty e^{-\frac{q^2}{4}(l^2-4iD\tau)}\frac{\sin(qr)}{qr}4\pi q^2 \mathrm{d}q\right\} \tag{SM-53}$$

where the integral is nothing but the Fourier-transform of a Gaussian function

$$\int_0^\infty e^{-aq^2}\frac{\sin(qr)}{qr}4\pi q^2 dq = \left(\frac{\pi}{a}\right)^{3/2}\exp[-r^2/(4a)] \tag{SM-54}$$

with $a = l^2/4 - iD\tau$. This leads to

$$g_W(r,\tau) = \frac{\exp\left[-\frac{(r/l)^2}{1+[4D\tau/l^2]^2}\right]}{\left(1+[4D\tau/l^2]^2\right)^{3/4}}\cos\left[\frac{(r/l)^2 4D\tau/l^2}{1+[4D\tau/l^2]^2} - \frac{3}{2}\tan^{-1}\left[\frac{4D\tau}{l^2}\right]\right] \tag{SM-55}$$

which proves Eq. (37) of the main text.

## V. DYNAMIC MODEL 3: $g_W(r,\tau)$ FOR STATIC FIELD GRF-4 (DEFORMATION MODE)

We derive here the field correlation function $g_W(r,\tau)$ for dynamic model 3, in the particular case where the static field is described by the elementary wave given in Eq. (59) of the main text. All static properties of this field are reported in Tab. I of the main text, under the label GRF-4. In particular, the spectral density is

$$f_W(q) = \left(\frac{l}{\sqrt{\pi}}\right)^3 \frac{1}{480}(ql)^4 e^{-[ql]^2/4} \tag{SM-56}$$

and the static correlation function is

$$g_W(r) = \left[1 - \frac{4}{3}\left(\frac{r}{l}\right)^2 + \frac{4}{15}\left(\frac{r}{l}\right)^4\right] e^{-[r/l]^2} \tag{SM-57}$$

We now consider successively the cases of ballistic and diffusive wave propagation.

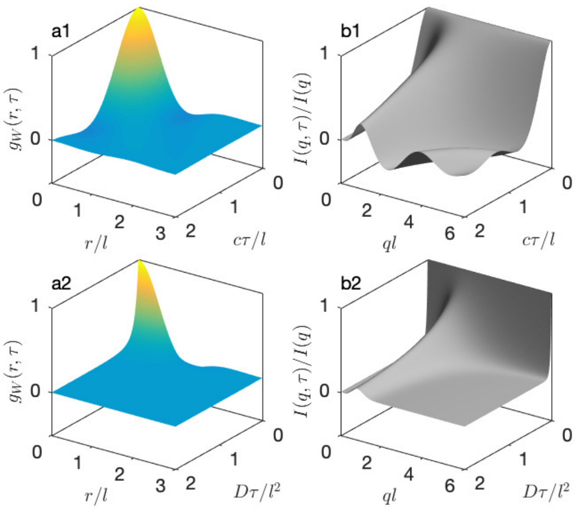


FIG. SM-11: Correlation function $g_W(r,\tau)$ of dynamic model 3 for static Gaussian fields GRF-4 of Tab I (main text) with (a1) ballistic and (a2) diffusive motion of elementary waves, together with corresponding intermediate scattering functions (b1 and b2) for clipping threshold $\alpha = 0$.

## A. Ballistic wave propagation

In the case of ballistic motion of elementary waves, the dynamic correlation function is obtained from Eq. (41) of the main text, by equating $\theta\langle A^2\rangle K(r)$ to $g_W(r)$ in Eq. (SM-57). This leads to

$$g_W(r,\tau) = \exp\left[-\left(\frac{r-c\tau}{l}\right)^2\right]\left\{\frac{16}{15}\left(\frac{rc\tau}{l^2}\right)^2 M_2\left[2\frac{rc\tau}{l^2}\right]\right.$$
$$+\frac{8}{15}\frac{rc\tau}{l^2}\left[5-2\left(\frac{r^2+(c\tau)^2}{l^2}\right)\right]M_1\left[2\frac{rc\tau}{l^2}\right]$$
$$\left.+\left[1-\frac{4}{3}\left(\frac{r^2+(c\tau)^2}{l^2}\right)+\frac{4}{15}\left(\frac{r^2+(c\tau)^2}{l^2}\right)^2\right]M_0\left[2\frac{rc\tau}{l^2}\right]\right\} \tag{SM-58}$$

where the function $M_n(a)$ is defined as

$$M_n(a) = \frac{e^{-a}}{2}\int_{-1}^{+1}\mu^n e^{+a\mu}\mathrm{d}\mu \tag{SM-59}$$

For $n=0$ to $n=2$, the values are

$$M_0(a) = \frac{1-e^{-2a}}{2a} \tag{SM-60}$$

$$M_1(a) = \frac{(a-1)+(a+1)e^{-2a}}{2a^2} \tag{SM-61}$$

$$M_2(a) = \frac{(a^2-2a+2)-(a^2+2a+2)e^{-2a}}{2a^3} \tag{SM-62}$$

The field correlation function is plotted in Fig. SM-11a1.

## B. Diffusive wave propagation

In the case of diffusive wave propagation, the correlation function $g_W(r,\tau)$ is conveniently calculated from the spectral density in Eq. (SM-56) through Eqs. (45) and (47) of the main text.

Starting from the expression for the 3D Fourier transform of a Gaussian function, namely

$$\int_0^\infty 4\pi q^2 dq \frac{\sin(qr)}{qr}\exp[-aq^2] = \left(\frac{\pi}{a}\right)^{3/2}\exp[-r^2/(4a)] \tag{SM-63}$$

and evaluating the derivative twice with respect to $a$, one obtains the following identity

$$\int_0^\infty 4\pi q^2 dq \frac{\sin(qr)}{qr}q^4\exp[-aq^2] = \frac{15\pi^{3/2}}{4a^{7/2}}\left(1-\frac{r^2}{3a}+\frac{r^4}{60a^2}\right)\exp[-r^2/(4a)] \tag{SM-64}$$

The field correlation function results then directly from Eqs. (45) and (47), by particularizing this identity to $a = l^2 + 4D\tau$, namely

$$g_W(r,\tau) = \left(1 + \frac{4D\tau}{l^2}\right)^{-7/2} \left\{1 - \frac{4}{3}\frac{r^2}{l^2 + 4D\tau} + \frac{4}{15}\left(\frac{r^2}{l^2 + 4D\tau}\right)^2\right\} \exp\left[\frac{-r^2}{l^2 + 4D\tau}\right] \tag{SM-65}$$

The field correlation function is plotted in Fig. SM-11a2.

## VI. ASYMPTOTIC EXPANSION OF THE INTERMEDIATE SCATTERING FUNCTION

The relation between the large-$q$ behaviour of $I(q,\tau)$ and the small-$r$ behaviour of the scattering length correlation function $C_\rho(r,\tau)$ (or of the covariances) is described by a general theorem by Lighthill, which generalizes the Riemann-Lebesgue lemma (ref. 42 of the main text). We provide here a less general and more accessible derivation, that is sufficient for our purpose in the main text.

Assuming 3D isotropy, the intermediate scattering function is written as

$$I(q,\tau) = \frac{4\pi}{q} \int_0^\infty dr\ rC_\rho(r,\tau)\ \sin(qr) \tag{SM-66}$$

Following a classical procedure (e.g. refs. 40-41 of the main text), the asymptotic behavior of $I(q,\tau)$ for large $q$ can be obtained by integrating the Fourier transform by parts. Before proceeding it is useful to note that for Eq. (SM-66) to exist at all $C_\rho$ has to be integrable in $\mathbb{R}^3$, which means that $C_\rho$ decreases faster than $r^{-3}$ for $r \to \infty$. Moreover, $C_\rho$ is finite for $r \to 0$, and we assume that this is also the case for all its derivatives (which excludes fractal-like structures from the present analysis).

With these conditions in mind, integrating Eq. (SM-66) by parts successively leads to

$$\begin{aligned} I(q,\tau) = -\frac{4\pi}{q^2}\Big\{ &\Big[rC_\rho(r,\tau)\cos(qr)\Big]_0^\infty \\ &- \int_0^\infty dr\ (C_\rho(r,\tau) + rC_\rho^{(1)}(r,\tau))\ \cos(qr)\Big\} \\ = \frac{4\pi}{q^3}\Big\{ &\Big[(C_\rho(r,\tau) + rC_\rho^{(1)}(r,\tau))\sin(qr)\Big]_0^\infty \\ &- \int_0^\infty dr\ (2C_\rho^{(1)}(r,\tau) + rC_\rho^{(2)}(r,\tau))\ \sin(qr)\Big\} \\ = \frac{4\pi}{q^4}\Big\{ &\Big[(2C_\rho^{(1)}(r,\tau) + rC_\rho^{(2)}(r,\tau))\cos(qr)\Big]_0^\infty \\ &- \int_0^\infty dr\ (3C_\rho^{(2)}(r,\tau) + rC_\rho^{(3)}(r,\tau))\ \cos(qr)\Big\} \end{aligned} \tag{SM-67}$$

where we use the notation $C_\rho^{(i)}(r,\tau)$ for the $i^{th}$ derivative of $C_\rho(r,\tau)$ with respect to $r$

$$C_\rho^{(i)}(r,\tau) = \frac{\partial^i C_\rho(r,\tau)}{\partial r^i} \tag{SM-68}$$

In the first two lines of Eq. (SM-67), the terms between square brackets vanish both for $r \to \infty$ and $r \to 0^+$, as a consequence of the limits mentioned in preamble. This is not the

case for the third line, so that one is left with

$$I(q,\tau) = -\frac{8\pi C_\rho^{(1)}(0^+,\tau)}{q^4} - \frac{4\pi}{q^4}\int_0^\infty dr\ \left(3C_\rho^{(2)}(r,\tau) + rC_\rho^{(3)}(r,\tau)\right)\ \cos(qr) \tag{SM-69}$$

The first term corresponds to Porod's law, as in Eqs. (48-49) of the main text.

The integration by parts can be continued further, leading to

$$\begin{aligned}
&I(q,\tau) + \frac{8\pi C_\rho^{(1)}(0^+,\tau)}{q^4} \\
&= -\frac{4\pi}{q^5}\Big\{\Big[\left(3C_\rho^{(2)}(r,\tau) + rC_\rho^{(3)}(r,\tau)\right)\ \sin(qr)\Big]_0^\infty \\
&\qquad\qquad - \int_0^\infty dr\ \left(4C_\rho^{(3)}(r,\tau) + rC_\rho^{(4)}(r,\tau)\right)\ \sin(qr)\Big\} \\
&= -\frac{4\pi}{q^6}\Big\{\Big[\left(4C_\rho^{(3)}(r,\tau) + rC_\rho^{(4)}(r,\tau)\right)\ \cos(qr)\Big]_0^\infty \\
&\qquad\qquad - \int_0^\infty dr\ \left(5C_\rho^{(4)}(r,\tau) + rC_\rho^{(5)}(r,\tau)\right)\ \cos(qr)\Big\}
\end{aligned} \tag{SM-70}$$

Here again the term between square brackets on the first line vanishes, but not on the second line. This leads to

$$\begin{aligned}
I(q,\tau) = &-\frac{8\pi C_\rho^{(1)}(0^+,\tau)}{q^4} + \frac{16\pi C_\rho^{(3)}(0^+,\tau)}{q^6} \\
&+ \frac{4\pi}{q^6}\int_0^\infty dr\ \left(5C_\rho^{(4)}(r,\tau) + rC_\rho^{(5)}(r,\tau)\right)\ \cos(qr)
\end{aligned} \tag{SM-71}$$

When this procedure is continued, the intermediate scattering function is approximated as a series of inverse even powers of $q$ (starting from $q^{-4}$), with coefficients proportional to the odd derivatives of $C_\rho$ for $r \to 0^+$. Note that for $q \to \infty$, the first terms are dominant in the series.

In the event where all odd derivatives of $C_\rho(r,\tau)$ with respect to $r$ would vanish at $r \to 0^+$, the intermediate scattering function decreases asymptotically with $q$ faster than any power law.

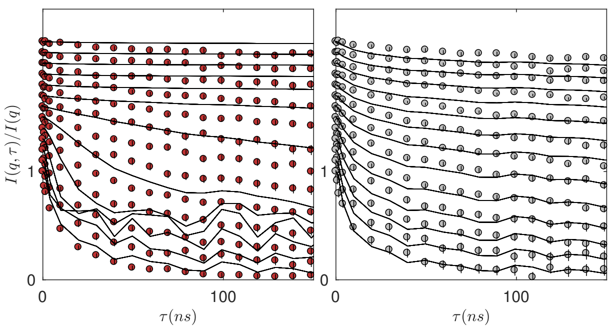


FIG. SM-12: 2D representation of the same NSE data and model as in Fig. 13 of the main text. The dots are the data in bulk (left) and film (right) contrasts, and the lines is the model with Eq. (61) as a dispersion relation. Each $q$ series is shifted vertically for clarity.

## VII. INFLUENCE OF NUMERICAL PARAMETERS ON THE SANS AND NSE ANALYSIS OF THE EMULSION

### A. Shape of the dispersion relation

As an alternative to Eq. (61) of the main text, the following general form was also tested as a dispersion relation

$$\omega = a_1 q + a_2 q^2 + a_3 q^3 + a_4 q^4 \tag{SM-72}$$

where $a_1$ to $a_4$ are the adjustable parameters. As illustrated in Fig. SM-13 this fit leads to alternating signs of the coefficients $a_n$, in such a way to keep $\omega$ close to zero for small values of $q$. This is similar to a cutoff frequency. The

### B. Asymptotic exponent $\nu$ of the piecewise-linear spectral density

The numerical parameter $\nu$ is introduced in Eq. (SM-26) to describe the asymptotic shape of the spectral density for infinitely large values of $q$. There are several constraints on the values of $\nu$:

- The integrability of $f_W(q)$ demands $\nu > 3$.
- In many instances, it is desirable that the clipped structure has finite surface area. As the latter is inversely related to the characteristic length $l_W$ (Eq. 8 of the main text), the condition for finite surface area is $\nu > 5$.

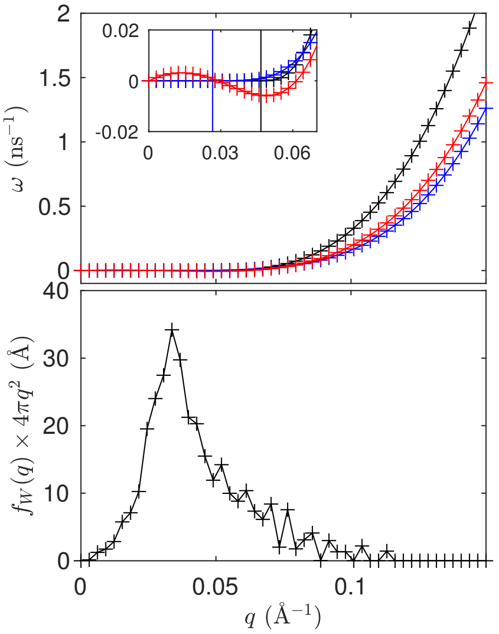


FIG. SM-13: Dispersion relations fitted to the NSE data (top), together with the spectral density in the form $4\pi q^2 f_W(q)$ (bottom). The models are Eq. (61) of the main text with exponent $n = 3$ (blue) and $n = 4$ (black), and Eq. (SM-72) (red). The inset is a magnified view highlighting the small$-q$ behaviour, with the cutoffs $q_c$ of the first two models.

- In the context of the dispersion-relation dynamics (model 2) with exponent $n$, the condition for observing a finite characteristic time $\tau_W$ is $\nu > 2n + 3$ (see Eq. 57 of the main text). In practice, the vertical slope in the NSE emulsion data point at a dynamics where $\tau_W$ is not defined. With the exponent $n = 3$, the condition on $\nu$ becomes $\nu < 9$.

Any value of $\nu$ intermediate between 5 and 9 yields a structure with finite surface area, and Brownian-like dynamics (with $\tau_W = 0$). The specific value chosen between these two bounds is relatively indifferent, as illustrated in Fig. SM-14 for $\nu = 5.1$ and $\nu = 8.9$. The corresponding values of the fitted parameter of the dispersion relation (Eq. 61 of the main text) are $a = 1980 \pm 150$ Å$^3$/ns and $q_c = 0.0465 \pm 0.0006$ Å$^{-1}$ (for $\nu = 5.1$) and $a = 2040 \pm 20$ Å$^3$/ns and $q_c = 0.0465 \pm 0.0002$ Å$^{-1}$ (for $\nu = 8.9$).

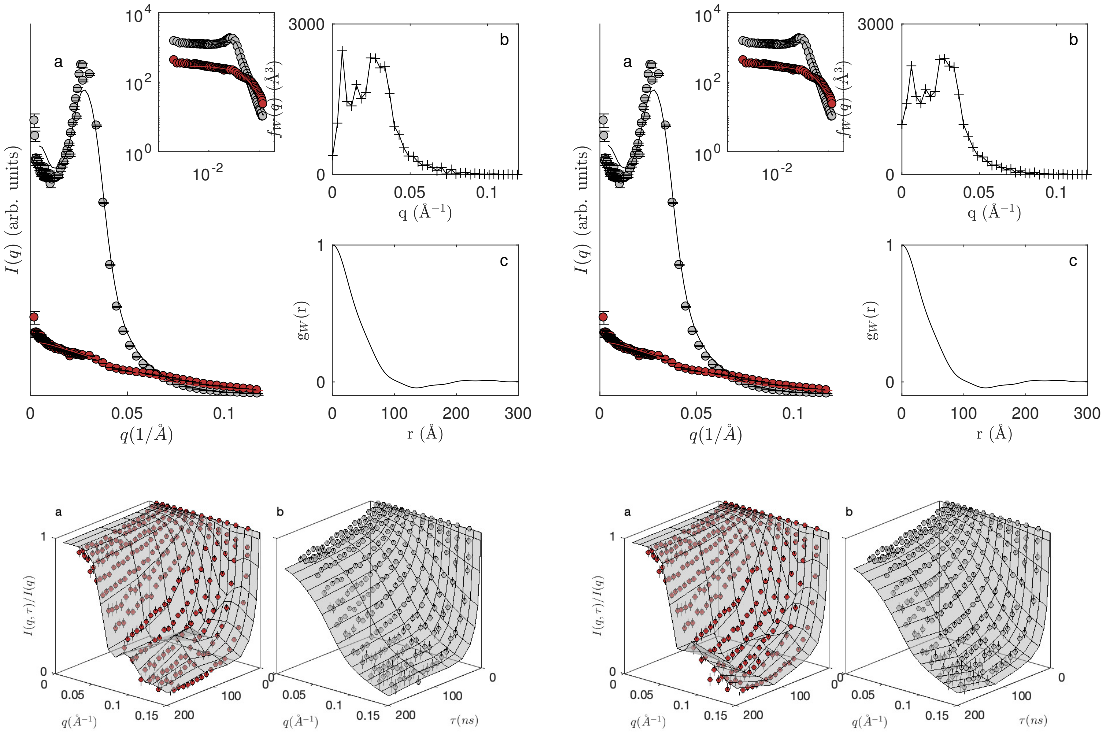


(a) $\nu = 5.1$ (b) $\nu = 8.9$

FIG. SM-14: Effect of parameter $\nu$ on the SANS (top) and NSE (bottom) analysis (for the piecewise-linear model with $M = 50$ nodes). The insets of the top figures are identical to Fig. SI-10, and those of the bottom figures to Fig. 13 of the main text.

## C. Number of $q$ values

Fig. SM-15 illustrates the influence of the number of $q$ series for the fitting of the NSE data with the dispersion relation in Eq. (61) of the main text. This figure is to be compared with Fig. 13 of the main text (in all cases $N = 50$ nodes and $\nu = 6$).

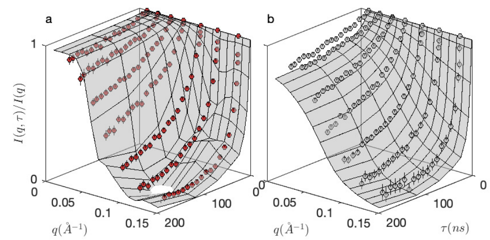

(a) $N_q = 7$: $a = 1920 \pm 20$ Å$^3$/ns and $q_c = 0.0447 \pm 0.0003$ Å$^{-1}$

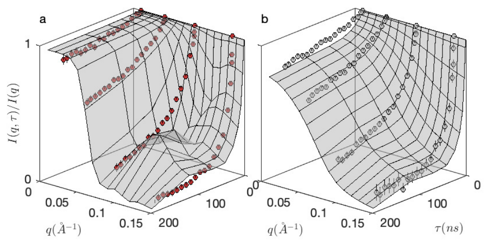

(b) $N_q = 4$: $a = 2060 \pm 150$ Å$^3$/ns and $q_c = 0.0475 \pm 0.0005$ Å$^{-1}$

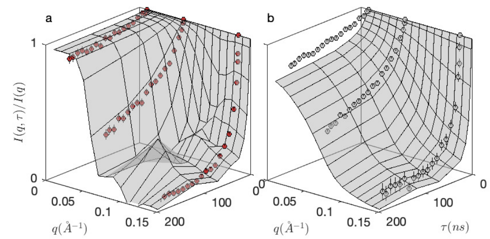

(c) $N_q = 3$: $a = 1850 \pm 60$ Å$^3$/ns and $q_c = 0.0426 \pm 0.0003$ Å$^{-1}$

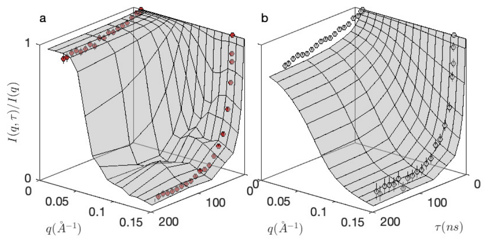

(d) $N_q = 2$: $a = 2120 \pm 160$ Å$^3$/ns and $q_c = 0.0459 \pm 0.0005$ Å$^{-1}$

FIG. SM-15: Impact of $N_q$ the number of $q$ series for the fitting of the NSE data with the dispersion relation in Eq. (61) (compare with Fig. 13 of the main text). The values of the fitted parameters are reported under each graph.
